# Supplementary material for: Cross-Domain Adaptive Teacher for Object Detection
Source: arXiv:2111.13216 source file (2022-05-11)
Supplement: Supplementary file 1 [file appendix.tex]

\subsection{Qualitative comparison}
To further justify the effectiveness of our propose adaptive unbiased teacher (AUT), we present the qualitative results of object detection on the testing set in Figure~\ref{fig:foggy}, Figure~\ref{fig:clipart1k}, and Figure~\ref{fig:water2k}. We compare our AUT with Source (F-RCNN) model and Oracle (F-RCNN) model. For the setting of weather adaptation, we can observe that there are many missing detections on source model when the fog is serious. Yet, our model is able to achieve the comparable detection result than Oracle model, which demonstrates our model is able to handle domain bias successfully without supervision on target domain. For the setting of real to artistic adaptation, both the Source (F-RCNN) model and Oracle (F-RCNN) model shows missing or incorrect detections in the two given samples. Our AUT instead produce more correct detected bounding boxes than both of the models.

\begin{figure}[H]
  \centering
  \includegraphics[width=\linewidth]{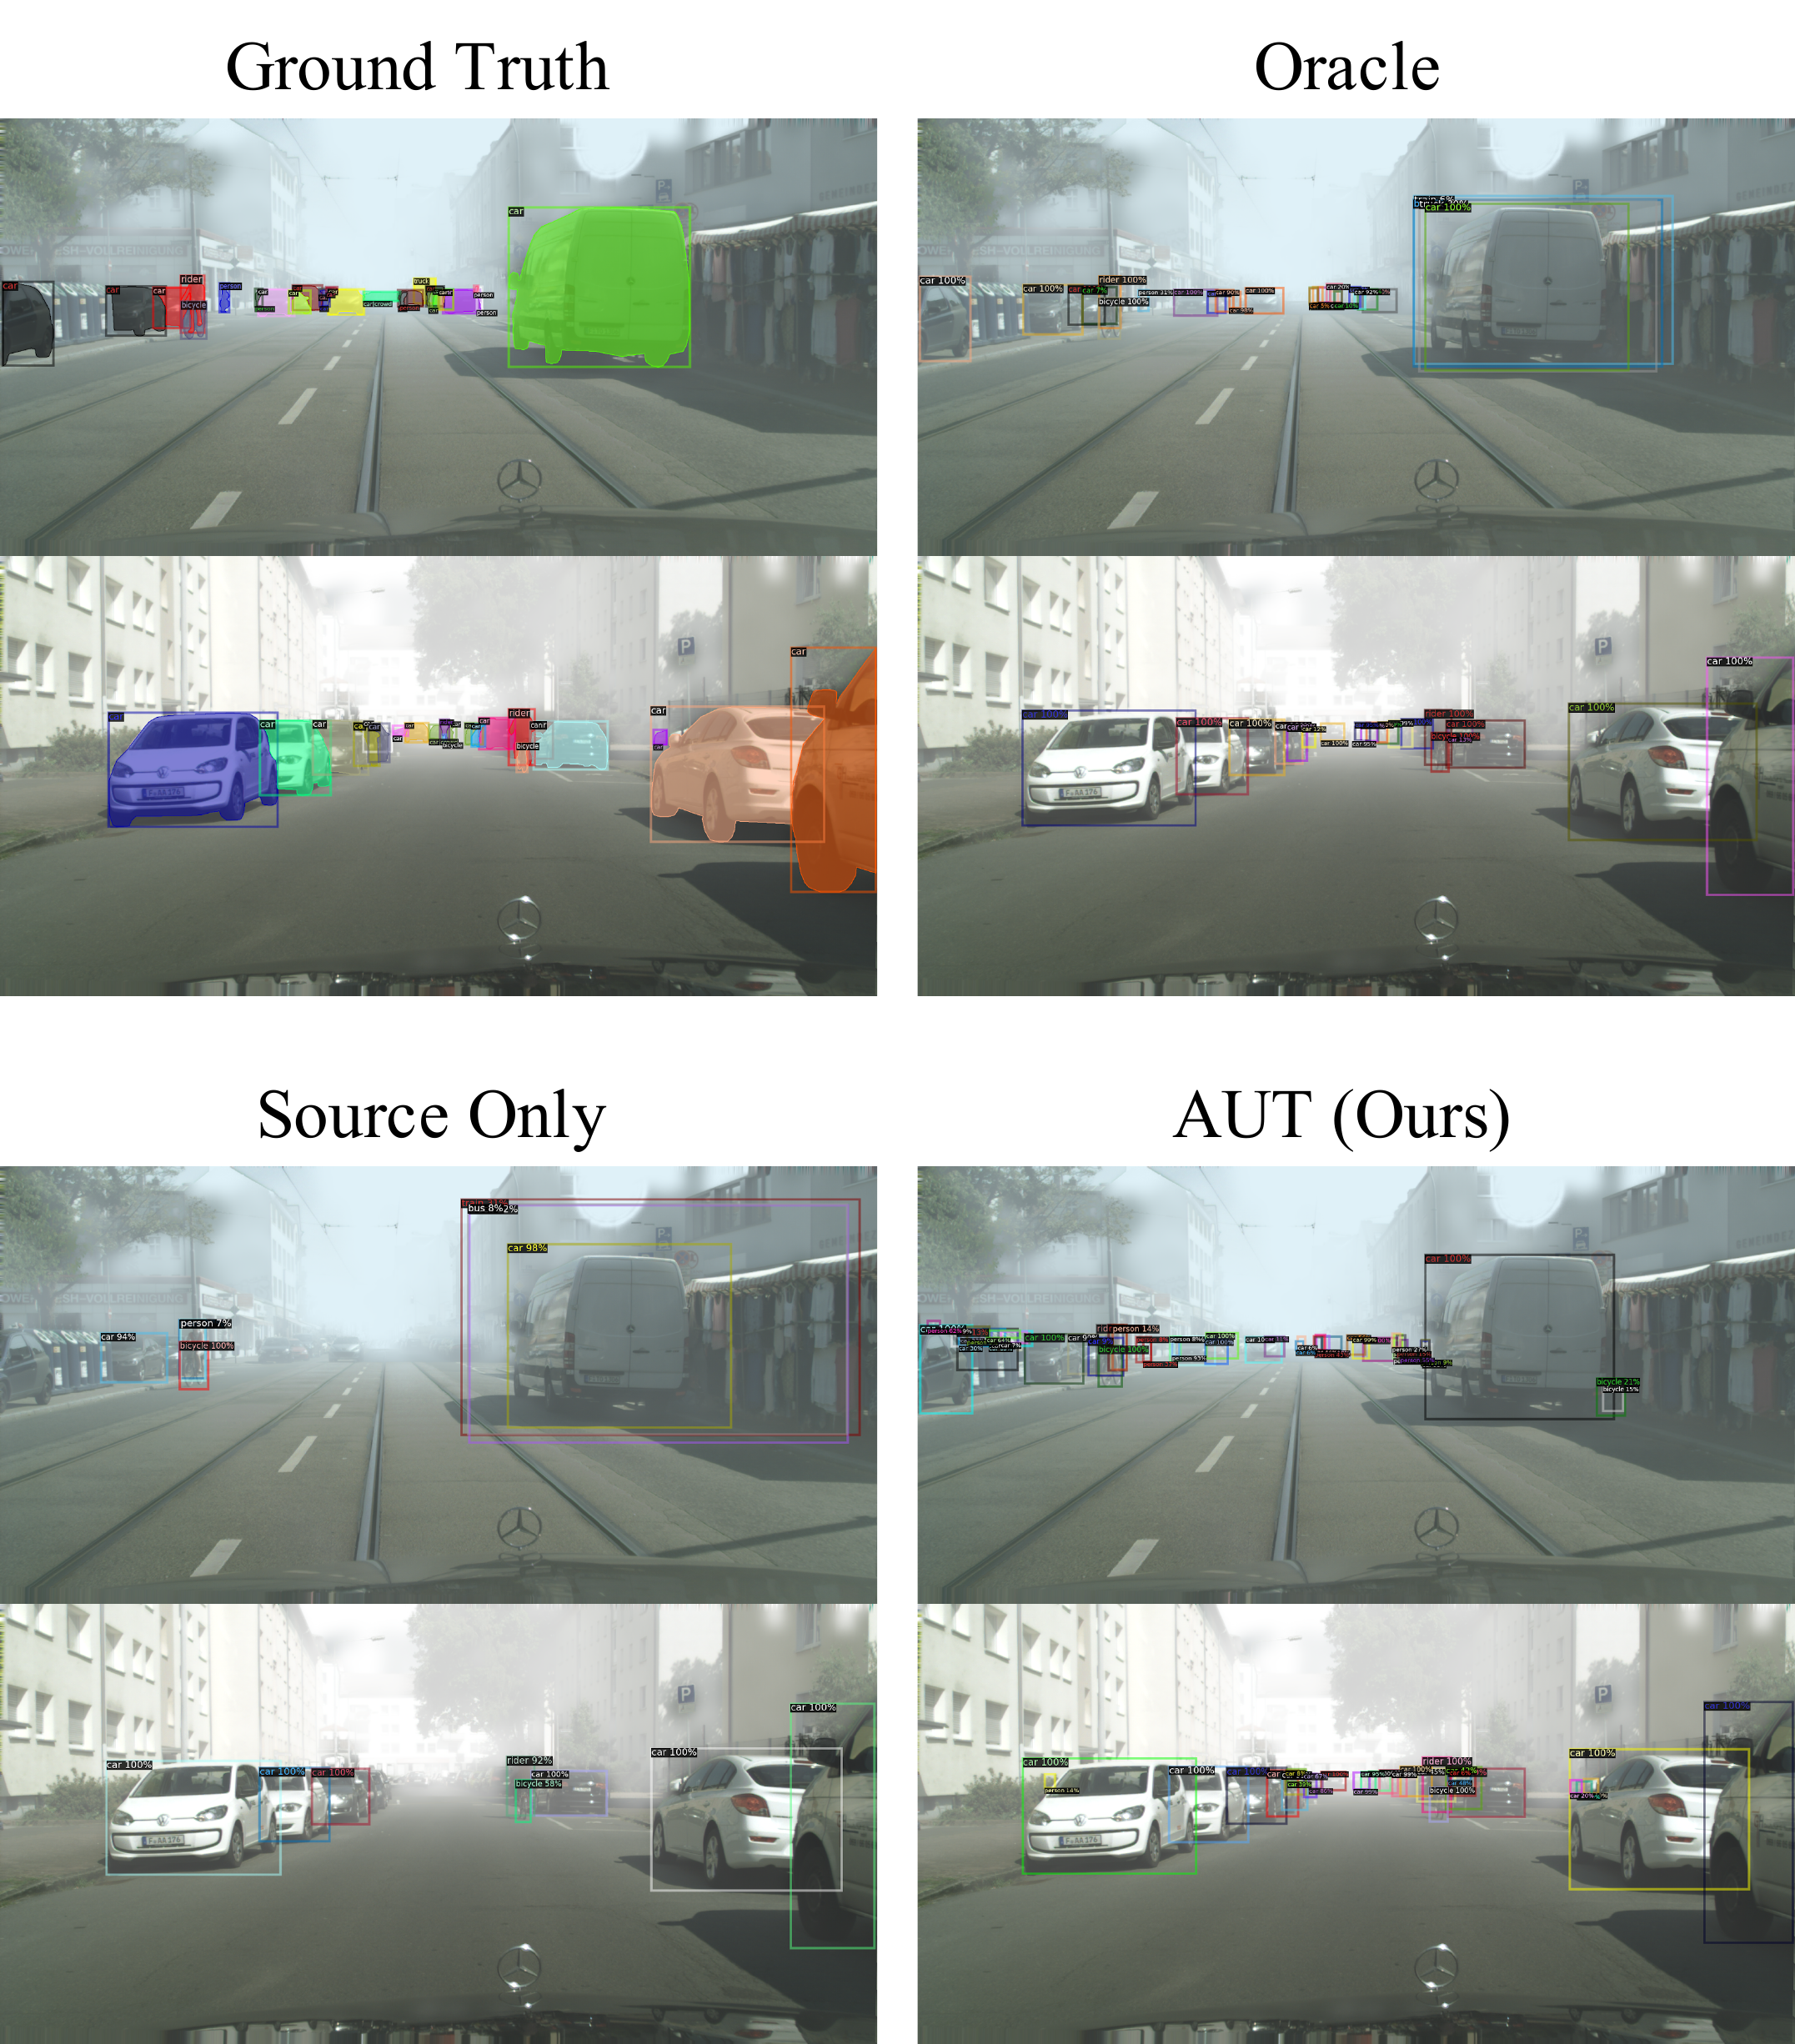}
  \caption{\textbf{Qualitative results and comparisons on Foggy Cityscapes}.}
  \label{fig:foggy}
%   \vspace{-5mm}
\end{figure}

\begin{figure}[H]
  \centering
  \includegraphics[width=0.7\linewidth]{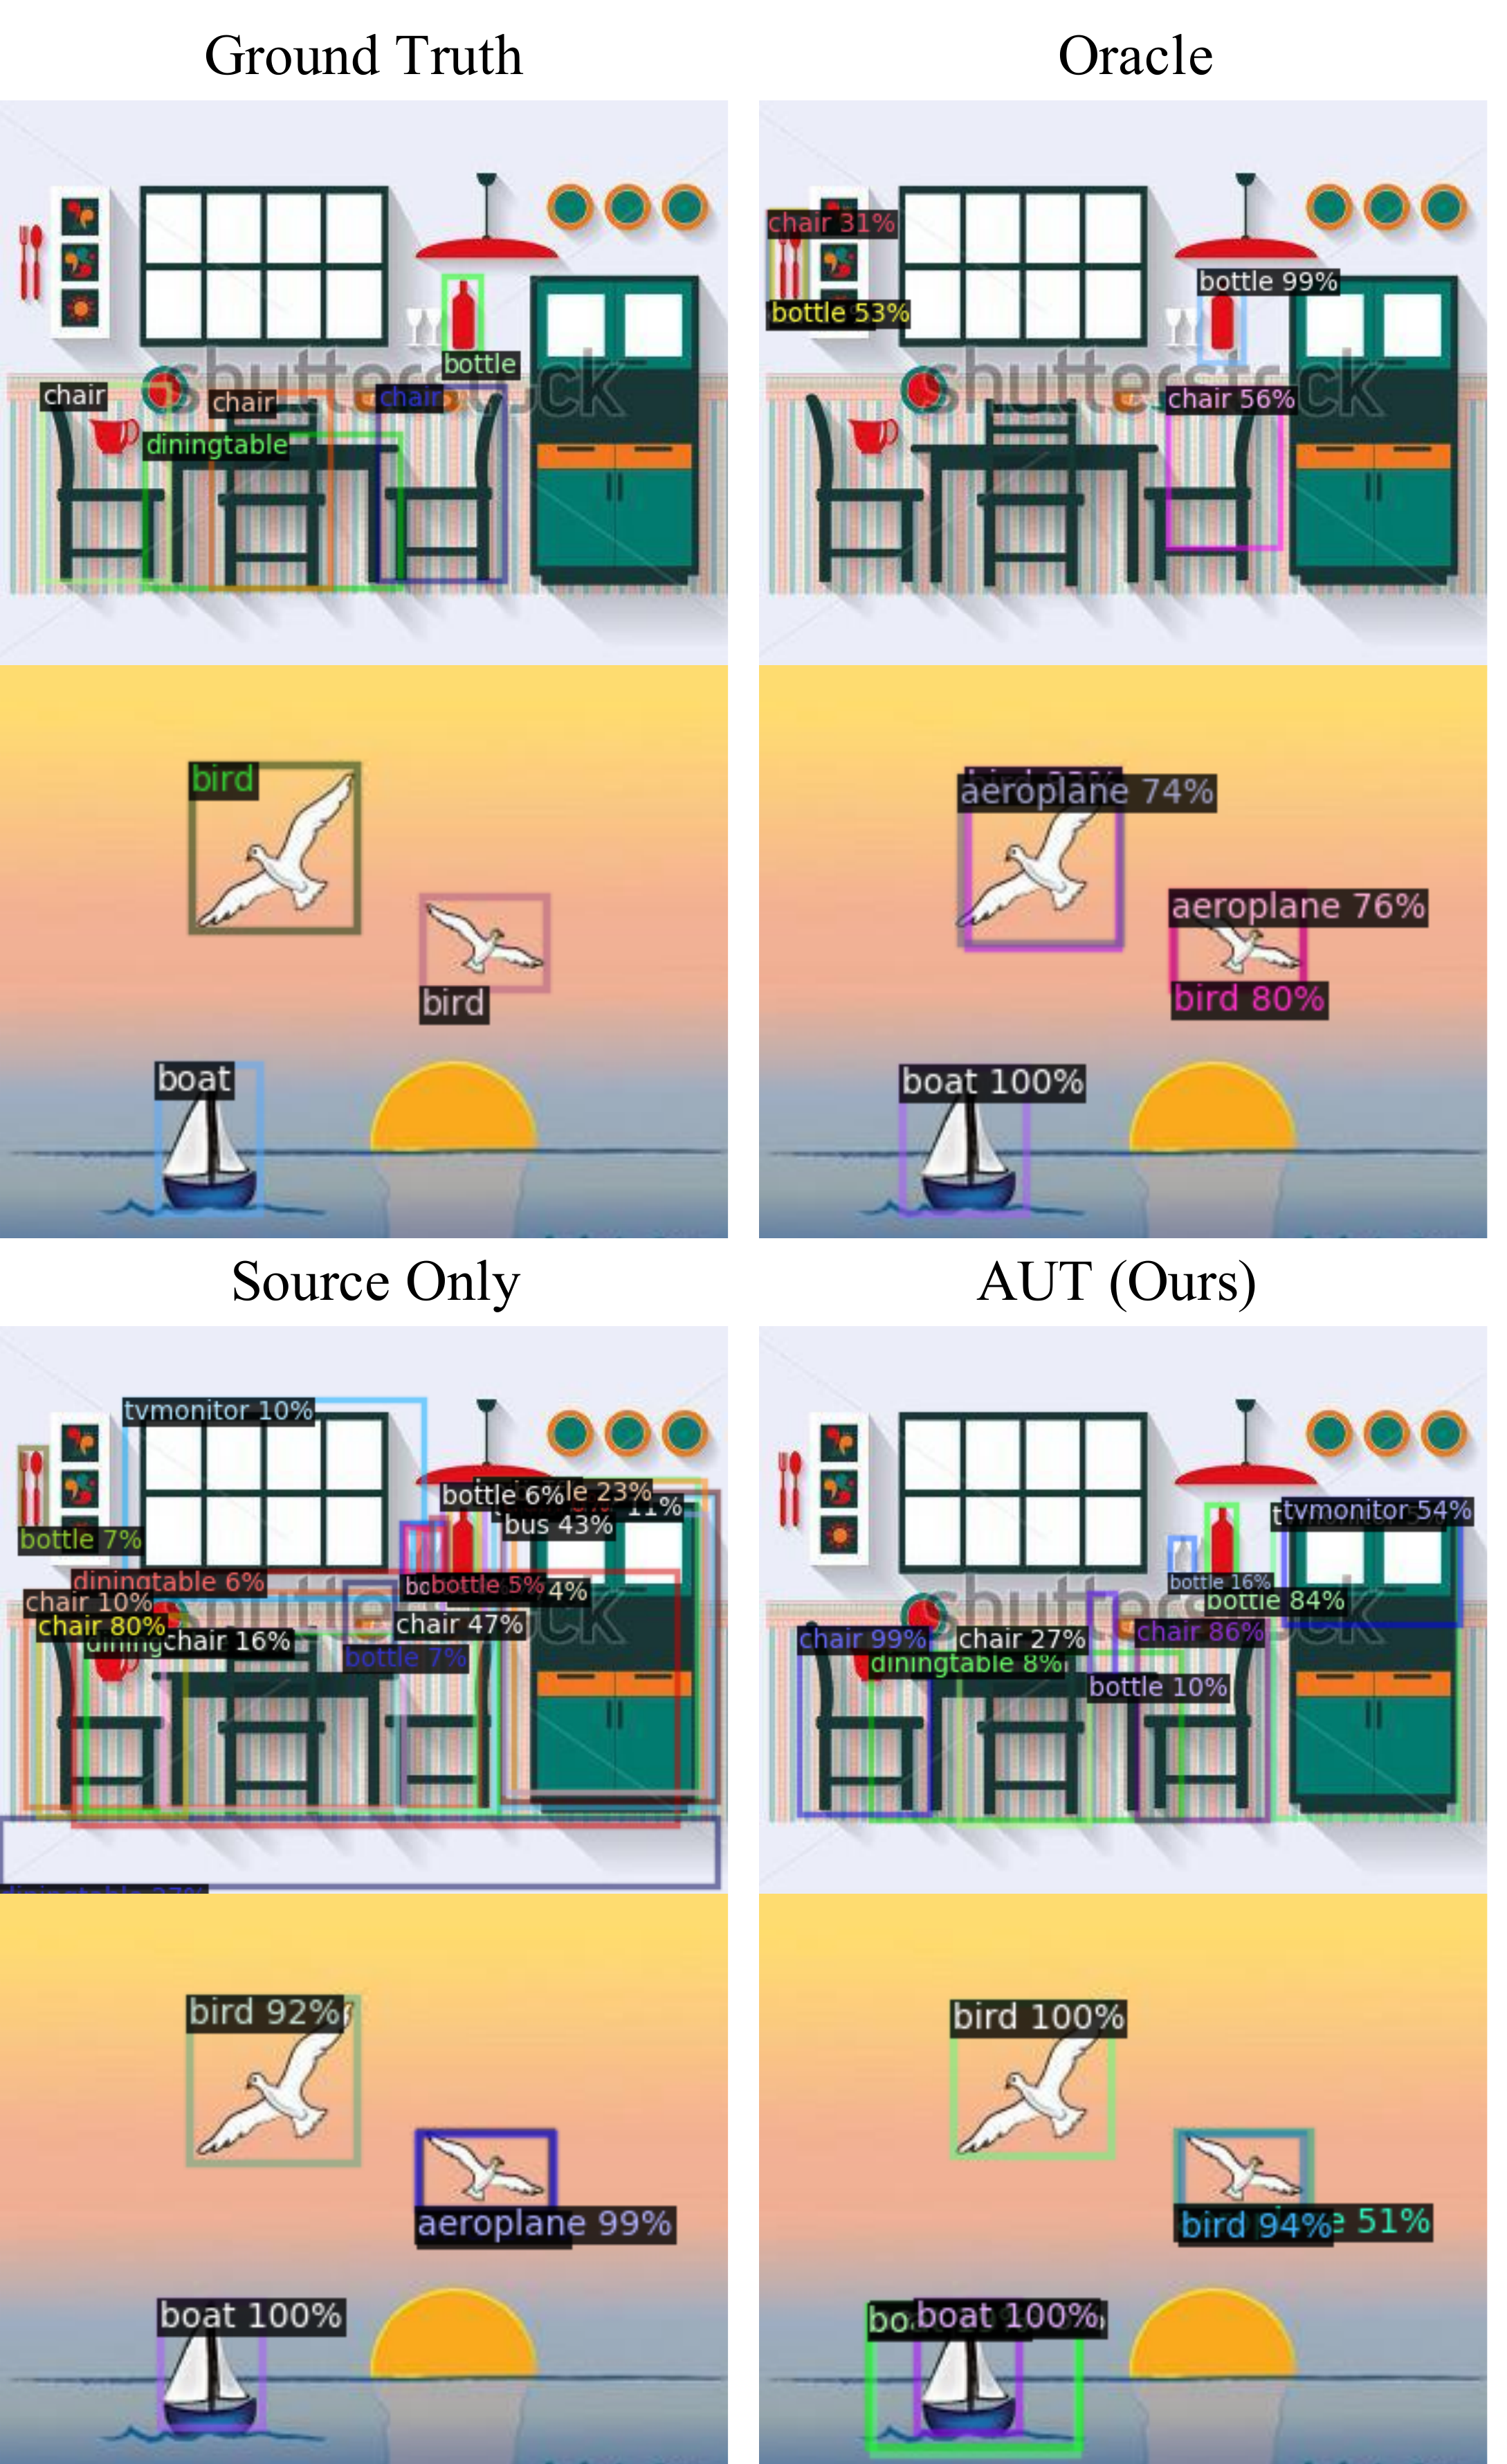}
  \caption{\textbf{Qualitative results and comparisons on Clipart1k}.}
  \label{fig:clipart1k}
%   \vspace{-5mm}
\end{figure}

\begin{figure}[H]
  \centering
  \includegraphics[width=0.65\linewidth]{fig/watercolor2.pdf}
  \caption{\textbf{Qualitative results and comparisons on Watercolor2k}. }
  \label{fig:water2k}
%   \vspace{-5mm}
\end{figure}

\subsection{More ablation studies}

We also analyze the weight $\lambda_{dis}$ of the adversarial loss $\mathcal{L}_{dis}$ in in Figure~\ref{fig:curve}. 
% Some phenomenons can be observed in this figure in two folds. 
We can see that, first, increasing weights can lead to improved performance, which supports the effectiveness of the discriminator in our model. Second, we see that with a sufficient weight of discriminator loss, the model will be able to have satisfactory performance. Third, the performance with the adversarial loss $\mathcal{L}_{dis}$ shows to be stable without decreasing drastically as the one without the loss.

% \begin{figure}[H]
%   \centering
%   \includegraphics[width=0.95\linewidth]{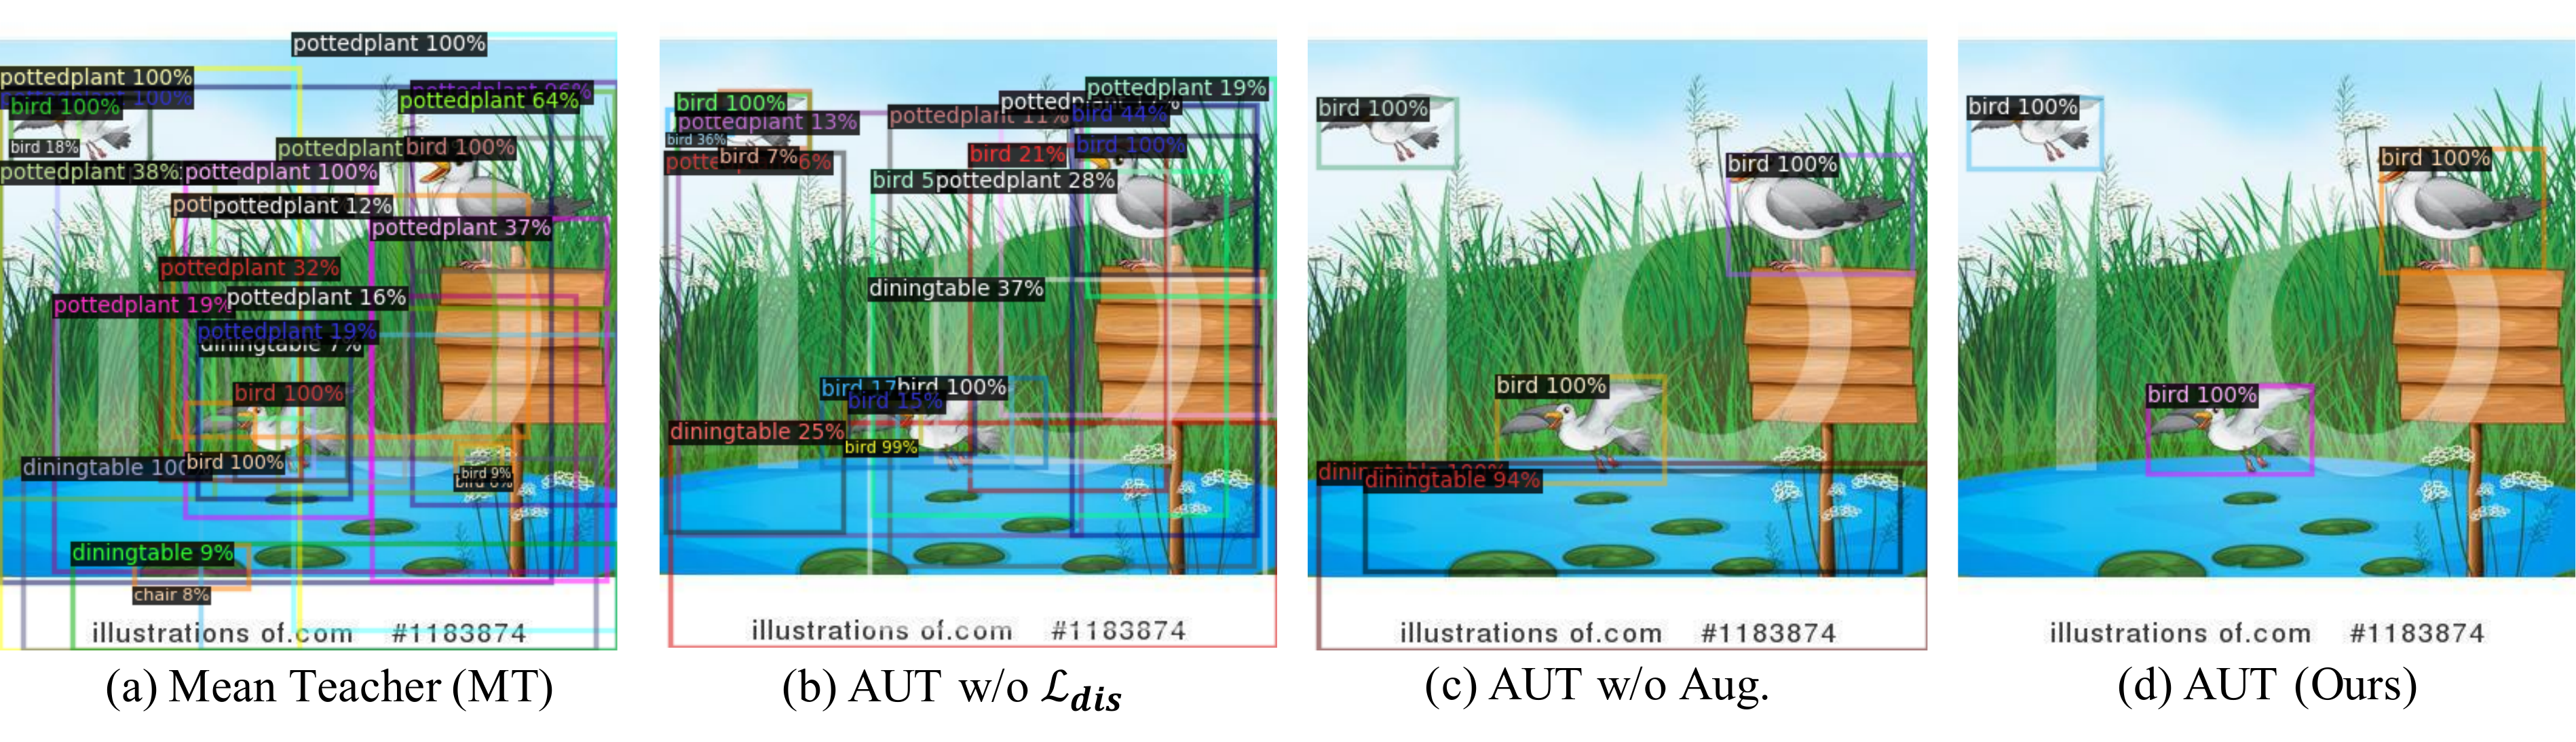}
%   \caption{\textbf{Qualitative ablation studies on Clipart1k}. This figure show the importance of adversarial loss $\mathcal{L}_{dis}$ and strong augmentation on student model.}
%   \label{fig:exp_quali_loss}
% %   \vspace{-5mm}
% \end{figure}

\begin{figure}[H]
  \centering
  \includegraphics[width=0.7\linewidth]{fig/Learning curve.pdf}
  \caption{\textbf{Mutual Learning curve on Clipart1k dataset}. Increasing weights of $\lambda_{dis}$ can achieve improved performance and stable learning curve.}
  \label{fig:curve}
\end{figure}
